# Supplementary material for: Laboratory photo-chemistry of covalently bonded fluorene clusters: observation of an interesting PAH bowl-forming mechanism
Source: arXiv:1901.03325 source file (2019-01-10)
Supplement: Supplementary file 1 [file SI.pdf]

Draft version January 8, 2019
Preprint typeset using LaTeX style emulateapj v. 12/16/11

# LABORATORY PHOTO-CHEMISTRY OF FLUORENE CLUSTERS: OBSERVATION OF A NEW PAH BOWL-FORMING MECHANISM

Weiwei Zhang[1,2,a], Yubing Si[3], Junfeng Zhen[1,2,*], Tao Chen[4,6], Harold Linnartz[5], Alexander G. G. M. Tielens[6]
[1]CAS Key Laboratory for Research in Galaxies and Cosmology, Department of Astronomy, University of Science and Technology of China, Hefei 230026, China
[2]School of Astronomy and Space Science, University of Science and Technology of China, Hefei 230026, China
[3]Henan Provincial Key Laboratory of Nanocomposites and Applications, Institute of Nanostructured Functional Materials, Huanghe Science and Technology College, Zhengzhou 450006, China
[4]Department of Theoretical Chemistry and Biology, School of Biotechnology, Royal Institute of Technology, 10691 Stockholm, Sweden
[5]Sackler Laboratory for Astrophysics, Leiden Observatory, Leiden University, P.O. Box 9513, 2300 RA Leiden, The Netherlands and
[6]Leiden Observatory, Leiden University, P.O. Box 9513, 2300 RA Leiden, The Netherlands

## 1. EXPERIMENTAL METHODS

The experimental setup i−PoP - instrument for Photodynamics of PAHs - was described in detail before (Zhen et al. 2014a), and only a brief description is given here. The neutral PAH molecules are evaporated by heating a high purity PAH powder in a special high temperature oven until they slowly start evaporating. The temperature of the oven ranges from 290 to 870 K, depending on the sublimation temperature of the PAHs under investigation. An electron gun is applied to ionize the molecules. As a byproduct, some of the highly excited PAHs may also lose an H-atom.

A steel mesh (hole diameter $\sim$ 0.1 mm) is mounted on top of the oven to increase the local density of molecules, ions, and fragments. The increased density facilitates cluster formation. Once formed, cation species are transported into the ion trap via an ion gate. Prior to ion injection, Helium buffer gas is introduced into the trap. The working pressures in the quadrupole ion trap and time-of-flight (TOF) chambers are $\sim$ 8.0 x $10^{-7}$ and $\sim$ 3.0 x $10^{-8}$ mbar, respectively. The light source to irradiate the trapped ions is a tunable dye laser (LIOP-TEC, Quasar2-VN) pumped by a Nd:YAG laser (DCR3, Spectra Physics), operated at 10 Hz. The output of the pulsed dye laser (linewidth $\sim$ 0.2 $cm^{-1}$, pulse duration $\sim$ 5 ns) is guided horizontally through the ion trap. Experiments are performed at 595 nm. The laser pulse energy is measured by a power meter (Vector, H310) before the beam enters the vacuum chamber.

I−PoP operates at a typical frequency of 0.2 Hz, i.e., one full measuring cycle last 5 s. It is possible to accumulate photo-fragmentation products of multiple laser shots, thereby increasing the fragmentation yield. A high precision delay generator (SRS DG535) controls the full timing sequence. Each scan cycle begins with an empty ion trap. At the leading edge of the master trigger the ion gate opens, allowing the ion trap to fill for a certain amount of time with PAH ions that are continuously generated by evaporation and subsequent electron impact ionization. Once the ions are trapped, external electrical waveforms are applied to the end cap electrodes to isolate a specific mass/charge (m/z) species. After a short time delay (typically $\sim$ 0.2s), the ion cloud thermalizes to room temperature ($\sim$ 298K) by collisions with the He buffer gas, and as a direct consequence the diameter of the cloud shrinks. The laser beam shutter opens and the ion cloud is irradiated. During each cycle, the laser irradiation time is changed to one of the preprogrammed time periods. At the end of the irradiation, a negative square pulse is applied to the end cap, accelerating the ions out of the trap and into the field free TOF region where the resulting mass fragments are measured. A LABVIEW program automates the full data acquisition process.

## 2. THEORETICAL CALCULATION DETAILS

Our theoretical calculations are carried out using density functional theory (DFT). The dissociation energies, minimum and transition state energies presented in this work are calculated using the hybrid functional B3LYP (Becke 1992; Lee et al. 1988) as implemented in the Gaussian 16 program (Frisch et al. 2016). All structures are optimized using the 6-311++G(d,p) basis set. The vibrational frequencies are calculated for the optimized geometries to verify that these correspond to minima or first-order saddle points (transition states) on the potential energy surface (PES). We have taken the zero point vibrational energy (ZPVE) into account.

In addition, to valid B3LYP, we took the reactions from $C_{26}H_{18}^{+}$ to $C_{26}H_{16}^{+}$ (losing hydrogen atoms step by step) as an example to make a comparison of various functionals calculation results, namely B3LYP-D3 (dispersion correction), PBE (pure functional) and M06HF (hybrid meta-GGA functional). The latter two functionals have been demonstrated are able to give accurate description of hemolytic bond breaking(Reilly et al. 2016). Table 1 shows the hydrogen dissociation energies obtained with different functionals. Clearly, B3LYP predicts the similar results with PBE and B3LYP-D3, indicating the typical problem of hemolytic bond breaking is not important in the current charged species.

## 3. DFT STUDIES OF THE STRUCTURE OF THE FLUORENE DIMER AND TRIMER

Focusing on the most abundant dimer and trimer ions ($C_{26}H_{18}{}^{+}$ and $C_{39}H_{26}{}^{+}$), we conclude that the complexation from monomer to dimer or trimer occurs on the $sp^3$ hybridized carbon of the fluorene molecules (Lang et al. 2013). Since the density of natural and ionic fluorene is

jfzhen@ustc.edu.cn
[1] [a]Current address: Department of Mechanical and Nuclear Engineering, Pennsylvania State University, University Park, PA 16802, United States.

higher in the ionization zone of i-PoP, the possible formation pathway of dimer and trimer fluorene cations could be the interaction between dehydrogenated neutral and charged fluorenes. And also since loss of H from the fluorene cation has a dissociation energy of only $\sim$ 2.3 eV, which means the abundance of $C_{13}H_9{}^+$ is higher than $C_{13}H_{10}{}^+$. Additionally, consider the fact that hydrogen dissociating from $sp^3$ hybridized carbon atoms is much easier than that from aromatic ring, we expect the structure of $C_{26}H_{18}{}^+$ as bonded dimers (West et al. 2018). Alternatively, it has been shown that ionization of van der Waals clusters of acetylene results in barrier less formation of covalently bonded larger species (Stein et al. 2017) and a similar process may be at work here. Our theoretical study shows that the dimer structure consists of two mono-fluorenes connected by a C−C single bond (as $[C_{13}H_9{-}C_{13}H_9]^+$), where two $sp^3$ hybridized carbon atoms have one C-H bond on each one; the trimer structure is that of three mono-fluorenes connected by two C−C single bond (as $[C_{13}H_9{-}C_{13}H_8{-}C_{13}H_9]^+$), where three $sp^3$ hybridized carbon atoms have one C-H bonds on each one. The optimized carbon skeletons of these fluorene units are not in the same plane, but form a three-dimensional structure. The dimer and trimer radical cations contain aliphatic units, in agreement with our interpretation of the experimental photo-dehydrogenation results.

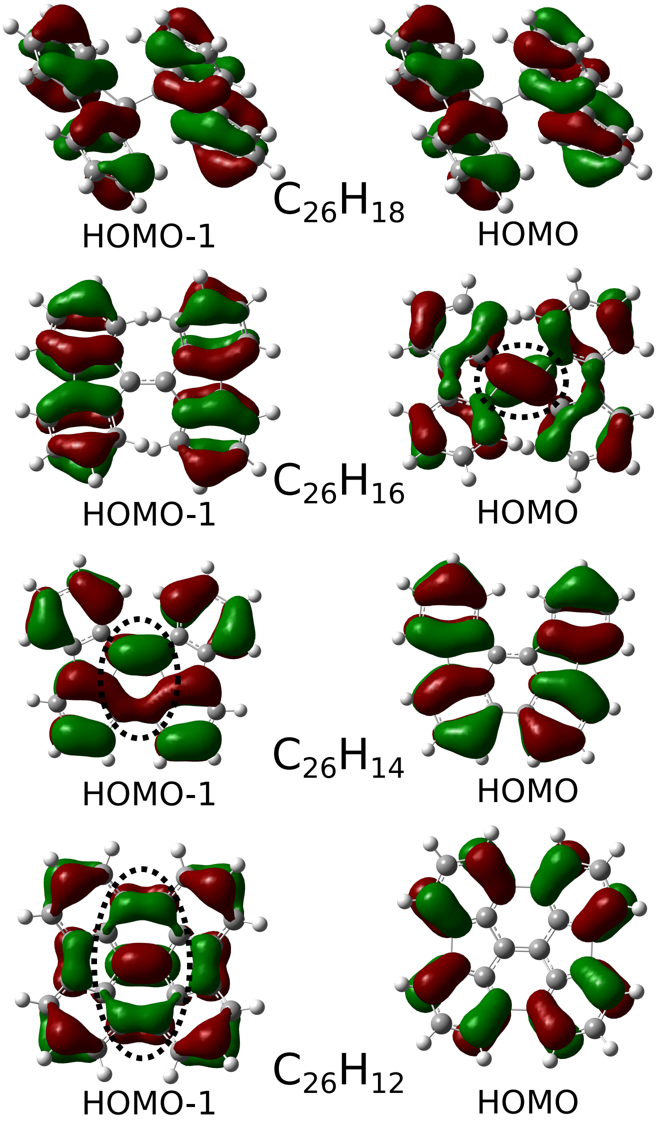


Fig. 1.— Highest occupied molecular $\alpha$ orbital (HOMO) and HOMO-1 for $C_{26}H_{18}{}^{+}$, $C_{26}H_{16}{}^{+}$, $C_{26}H_{14}{}^{+}$ and $C_{26}H_{12}{}^{+}$. It is found that there exists no conjugated $\pi$ bond between monomers in $C_{26}H_{18}{}^{+}$, while one, two and three conjugated C-C $\pi$ bonds are formed in $C_{26}H_{16}{}^{+}$, $C_{26}H_{14}{}^{+}$ and $C_{26}H_{12}{}^{+}$, respectively. The three newly formed conjugated $\pi$ bonds in $C_{26}H_{12}{}^{+}$ and the C-C $\pi$ bonds within each monomer can form large delocalized conjugated $\pi$ bonds.

TABLE 1

Hydrogen dissociation energies with different functionals using 6-311++G** basis set. The ZPVE has also been taken into account. (unit: eV)

| DFTs | $1^{st}$ H | $2^{nd}$ H |
|---|---|---|
| B3LYP | 2.337 | 2.614 |
| B3LYP-D3 | 2.456 | 2.695 |
| M06HF | 2.198 | 3.104 |
| PBE | 2.330 | 2.522 |

TABLE 2

Energies of all species, ZPVE is also included (unit: a.u.)

| Species | $E_{electronic}$ | ZPVE | $E_{total}$ |
|---|---|---|---|
| $C_{26}H_{18}{}^{+}$ | -1001.610774 | 0.354832 | -1001.255942 |
| $C_{26}H_{17}{}^{+}$ | -1001.011619 | 0.343754 | -1000.667862 |
| $C_{26}H_{16}{}^{+}$ | -1000.401314 | 0.331788 | -1000.069526 |
| TS1a | -1000.332864 | 0.329094 | -1000.00377 |
| $C_{26}H_{16}{}^{+}$-IMa | -1000.356317 | 0.332210 | -1000.024107 |
| TS2a | -1000.293678 | 0.323020 | -999.970658 |
| $C_{26}H_{15}{}^{+}$ | -999.7938721 | 0.3215941 | -999.472278 |
| $C_{26}H_{14}{}^{+}$ | -999.2126026 | 0.3091356 | -998.903467 |
| TS3a | -999.1023738 | 0.3091708 | -998.793203 |
| $C_{26}H_{14}{}^{+}$-IMa | -999.1072467 | 0.3104237 | -998.796823 |
| TS4a | -999.0198882 | 0.3019862 | -998.717902 |
| $C_{26}H_{12}{}^{+}$ | -997.9475467 | 0.2867287 | -997.660818 |
| $C_{39}H_{26}{}^{+}$ | -1501.938434 | 0.522934 | -1501.415500 |
| $C_{39}H_{24}{}^{+}$ | -1500.710374 | 0.498375 | -1500.211999 |
| $C_{39}H_{22}{}^{+}$ | -1499.496660 | 0.477539 | -1499.019120 |
| $C_{39}H_{20}{}^{+}$(1) | -1498.240186 | 0.454912 | -1497.785274 |
| $C_{39}H_{20}{}^{+}$(2) | -1498.307315 | 0.456046 | -1497.851270 |

## 4. COORDINATES FOR ALL SPECIES IN XYZ FORMAT

44
C26H18+:
C -2.204330 -0.263137 0.723233
C -1.365953 0.669289 0.134023
C -0.534651 0.569363 -1.135800
C 0.534651 -0.569363 -1.135800
C 1.365953 -0.669289 0.134023
C 2.204330 0.263137 0.723233
C 0.054536 1.965771 -1.237053
C -0.054536 -1.965771 -1.237053
C -0.872166 -2.505246 -2.214975
C 0.872166 2.505246 -2.214975
C 1.234896 -1.967141 0.701765
C 0.366589 -2.759652 -0.138056
C -1.234896 1.967141 0.701765
C -0.366589 2.759652 -0.138056
C -1.280241 -3.839047 -2.091055
C 1.280241 3.839047 -2.091055
C 2.889860 -0.090213 1.890686
C -2.889860 0.090213 1.890686
H 3.548183 0.630589 2.361538
H -1.918590 -4.275068 -2.850586
H 1.918590 4.275068 -2.850586
H -3.548183 -0.630589 2.361538
C 2.748393 -1.368186 2.463089
C -0.872166 -4.625735 -0.999867
C 0.872166 4.625735 -0.999867
C 0.047413 4.097615 -0.019442
C -1.927205 2.314186 1.875029
C -2.748393 1.368186 2.463089
C 1.927205 -2.314186 1.875029
C -0.047413 -4.097615 -0.019442
H 3.295181 -1.610096 3.366423
H 1.829257 -3.303365 2.306059
H 0.275971 -4.708337 0.815089
H -1.202162 -5.655388 -0.933597
H 1.202162 5.655388 -0.933597
H -0.275971 4.708337 0.815089
H -1.829257 3.303365 2.306059
H -3.295181 1.610096 3.366423
H -2.345543 -1.246257 0.292030
H 2.345543 1.246257 0.292030
H 1.195339 1.920083 -3.068952
H -1.195339 -1.920083 -3.068952
H 1.189504 -0.393612 -1.997460
H -1.189504 0.393612 -1.997460
43
C26H17+:
C -1.851188 -0.263007 1.137176
C -1.165104 0.740684 0.443297
C -0.052421 0.671471 -0.477930
C 0.741177 -0.515191 -0.884011
C 1.695209 -0.847622 0.280603
C 2.651317 -0.042450 0.886726
C 0.241631 2.013493 -0.913103
C -0.026335 -1.817979 -1.056084
C -1.030768 -2.116741 -1.966650
C 1.206087 2.476387 -1.814635
C 1.491459 -2.183307 0.684911
C 0.438007 -2.780175 -0.138307
C -1.537996 2.108015 0.598103
C -0.648723 2.916172 -0.266417
C -1.575779 -3.402389 -1.957442
C 1.282372 3.849042 -2.063672
C 3.433862 -0.593244 1.902497
C -2.890790 0.105705 1.995317
H 4.196355 0.010168 2.380013
H -2.351342 -3.661909 -2.668102
H 2.018847 4.233261 -2.757933
H -3.431079 -0.656401 2.542595
C 3.244556 -1.918959 2.305448
C -1.120973 -4.362795 -1.047198
C 0.408552 4.725365 -1.423655
C -0.571360 4.266447 -0.515366
C -2.566742 2.464592 1.437578
C -3.243254 1.444141 2.141563
C 2.279046 -2.722951 1.700969
C -0.111914 -4.063188 -0.134045
H 3.861166 -2.328119 3.097045
H 2.150522 -3.751914 2.016264
H 0.236451 -4.817228 0.562143
H -1.555455 -5.355448 -1.058498
H 0.478449 5.787490 -1.628621
H -1.237355 4.974827 -0.037464
H -2.863132 3.498531 1.567861
H -4.057275 1.711965 2.805220
H -1.594305 -1.305792 1.010577
H 2.803987 0.986076 0.579425
H 1.881969 1.795328 -2.318395
H -1.383884 -1.380187 -2.680259
H 1.315653 -0.285774 -1.785841
42
C26H16+:
C 1.267116 2.301079 1.067619
C 1.571295 1.086107 0.441104
C 0.708924 0.000000 0.000000
C -0.708924 0.000000 0.000000
C -1.571295 -1.086107 0.441104
C -1.267116 -2.301079 1.067619
C 1.571295 -1.086107 -0.441104
C -1.571295 1.086107 -0.441104
C -1.267116 2.301079 -1.067619
C 1.267116 -2.301079 -1.067619
C -2.925352 -0.674945 0.294036
C -2.925352 0.674945 -0.294036
C 2.925352 0.674945 0.294036
C 2.925352 -0.674945 -0.294036
C -2.313931 3.124308 -1.484681
C 2.313931 -3.124308 -1.484681
C -2.313931 -3.124308 1.484681
C 2.313931 3.124308 1.484681
H -2.095342 -4.070879 1.963169
H -2.095342 4.070879 -1.963169
H 2.095342 -4.070879 -1.963169
H 2.095342 4.070879 1.963169
C -3.639206 -2.730218 1.302032
C -3.639206 2.730218 -1.302032
C 3.639206 -2.730218 -1.302032
C 3.955928 -1.492048 -0.713834
C 3.955928 1.492048 0.713834
C 3.639206 2.730218 1.302032
C -3.955928 -1.492048 0.713834
C -3.955928 1.492048 -0.713834
H -4.440267 -3.379743 1.634892
H -4.991978 -1.192164 0.609555

H -4.991978 1.192164 -0.609555
H -4.440267 3.379743 -1.634892
H 4.440267 -3.379743 -1.634892
H 4.991978 -1.192164 -0.609555
H 4.991978 1.192164 0.609555
H 4.440267 3.379743 1.634892
H 0.241664 2.602255 1.239368
H -0.241664 -2.602255 1.239368
H 0.241664 -2.602255 -1.239368
H -0.241664 2.602255 -1.239368
42
TS1a:
C -0.579958 2.135194 0.718005
C -0.236732 0.867698 1.335973
C 0.015392 -0.396357 0.688748
C 0.067633 -0.388633 -0.713907
C -0.216443 -1.363297 -1.767888
C -0.532918 -2.719897 -1.722894
C 0.252396 -1.368137 1.754859
C 0.300922 0.869177 -1.363885
C 0.646304 2.128906 -0.716022
C 0.583204 -2.724924 1.731493
C -0.250462 -0.664409 -3.008903
C 0.037561 0.760744 -2.741706
C -0.058475 0.738174 2.728042
C 0.218420 -0.676174 3.001447
C 0.580984 3.293450 -1.595485
C 0.828362 -3.384852 2.935459
C -0.828451 -3.385572 -2.916556
C -0.573989 3.285891 1.593515
H -1.064860 -4.442324 -2.895361
H 0.844420 4.265077 -1.195501
H 1.078718 -4.438827 2.923684
H -0.851016 4.251395 1.186220
C -0.829255 -2.701650 -4.129871
C 0.295681 3.156550 -2.928608
C 0.764030 -2.705635 4.154602
C 0.470103 -1.340052 4.194051
C -0.065672 1.883463 3.516145
C -0.294549 3.156859 2.934316
C -0.551102 -1.325913 -4.184057
C 0.033110 1.891282 -3.539268
H -1.063433 -3.233762 -5.044250
H -0.586032 -0.802581 -5.132420
H -0.175708 1.842279 -4.600732
H 0.310818 4.038960 -3.558641
H 0.956824 -3.239698 5.077150
H 0.446836 -0.816884 5.143250
H 0.126348 1.820784 4.581961
H -0.296336 4.031575 3.573225
H -1.437115 2.119498 0.046533
H -0.566836 -3.259978 -0.786911
H 0.673420 -3.266889 0.800109
H 1.528239 2.109491 -0.075955
42
C26H16+-IMa:
C -0.100850 2.113240 0.728115
C 0.473355 0.984780 1.511107
C 1.174333 -0.124581 0.992941
C 1.410453 -0.133653 -0.405511
C 1.801169 -1.131132 -1.413398
C 2.041468 -2.501760 -1.334328
C 1.504963 -0.990910 2.134668
C 1.208359 1.082700 -1.091054
C 0.839308 2.390538 -0.483097
C 2.252682 -2.162416 2.238642
C 1.834529 -0.484649 -2.682456
C 1.433834 0.916511 -2.483720
C 0.348338 0.883878 2.922466
C 0.981127 -0.385224 3.312887
C 0.406330 3.395759 -1.508227
C 2.427534 -2.747537 3.495791
C 2.361255 -3.204004 -2.499635
C -0.504671 3.265750 1.598509
H 2.555071 -4.268352 -2.443449
H 0.017757 4.346773 -1.162789
H 3.002511 -3.661572 3.582285
H -0.838670 4.179021 1.119768
C 2.427197 -2.555639 -3.732176
C 0.604941 3.185926 -2.831396
C 1.878443 -2.168015 4.638861
C 1.158827 -0.969524 4.555960
C -0.171396 1.939093 3.630179
C -0.575693 3.142977 2.945402
C 2.150190 -1.186690 -3.833843
C 1.144802 1.948861 -3.341139
H 2.680624 -3.118494 -4.622443
H 2.178030 -0.697195 -4.800575
H 1.272693 1.839801 -4.412451
H 0.345689 3.961705 -3.542182
H 2.022358 -2.640785 5.602914
H 0.759164 -0.512679 5.454033
H -0.245497 1.906078 4.711550
H -0.938828 3.972280 3.540936
H -1.051951 1.741661 0.291438
H 1.962904 -3.035875 -0.398245
H 2.718075 -2.613425 1.373940
H 1.771532 2.811185 -0.050120
42
TS2a:
C -0.506132 1.951887 0.610832
C 0.072248 0.815042 1.350610
C 0.674961 -0.347674 0.801724
C 0.857317 -0.359133 -0.583888
C 1.358255 -1.310279 -1.575984
C 1.672312 -2.668280 -1.496410
C 1.032079 -1.209275 1.954246
C 0.568807 0.866320 -1.312387
C 0.028193 2.052449 -0.797565
C 1.708104 -2.422185 2.056369
C 1.445526 -0.641317 -2.833261
C 0.948487 0.735348 -2.662509
C 0.040290 0.747108 2.766076
C 0.622609 -0.544603 3.143592
C -0.203240 3.112658 -1.702736
C 1.927524 -2.979164 3.318982
C 2.117876 -3.334081 -2.639961
C -0.767458 3.151798 1.456923
H 2.362412 -4.387689 -2.583992
H -0.659966 4.035458 -1.367267
H 2.448181 -3.926045 3.397031
H -1.083044 4.067470 0.972289
C 2.242876 -2.658463 -3.852589
C 0.189768 2.986419 -3.027758
C 1.492658 -2.334835 4.476813
C 0.844972 -1.100859 4.396074
C -0.355689 1.854431 3.482791
C -0.740249 3.061959 2.811971

C 1.896388 -1.303960 -3.960134
C 0.770237 1.800392 -3.525563
H 2.595151 -3.190476 -4.728400
H 1.971623 -0.798307 -4.915588
H 1.052699 1.739424 -4.569837
H 0.039865 3.821014 -3.702309
H 1.669244 -2.788307 5.444562
H 0.528498 -0.591523 5.299119
H -0.342705 1.845700 4.567403
H -0.998157 3.926344 3.411948
H -1.557069 1.595462 0.440388
H 1.546384 -3.222713 -0.578764
H 2.087595 -2.935923 1.186721
H 1.768807 2.822505 -0.066051
41
C26H15+
C -0.508093 1.950220 0.611136
C 0.061981 0.809314 1.347105
C 0.653138 -0.359031 0.796806
C 0.835507 -0.367514 -0.588587
C 1.351690 -1.311903 -1.578052
C 1.685537 -2.665365 -1.496691
C 1.015239 -1.218137 1.951107
C 0.528970 0.857073 -1.322390
C -0.043843 2.023018 -0.820778
C 1.676768 -2.438960 2.055059
C 1.437604 -0.641255 -2.834966
C 0.923474 0.729941 -2.668404
C 0.049534 0.750780 2.763846
C 0.625370 -0.543001 3.141193
C -0.226720 3.098084 -1.701139
C 1.903610 -2.990227 3.318783
C 2.147642 -3.325141 -2.636931
C -0.759267 3.154620 1.453318
H 2.406073 -4.375310 -2.579542
H -0.677310 4.023926 -1.365176
H 2.413086 -3.943184 3.396808
H -1.081791 4.066854 0.966957
C 2.271295 -2.647018 -3.848168
C 0.188262 2.984625 -3.025695
C 1.489983 -2.333556 4.477482
C 0.855109 -1.093541 4.395202
C -0.323138 1.867109 3.479389
C -0.713263 3.072133 2.808594
C 1.906913 -1.297119 -3.957864
C 0.761565 1.800391 -3.528268
H 2.636545 -3.173753 -4.721915
H 1.981920 -0.790177 -4.912606
H 1.061008 1.746763 -4.568127
H 0.063623 3.831941 -3.689517
H 1.672094 -2.782882 5.446119
H 0.552869 -0.575007 5.297903
H -0.291658 1.864769 4.563690
H -0.962232 3.940034 3.407241
H -1.569953 1.599452 0.491166
H 1.561584 -3.222008 -0.580447
H 2.038705 -2.965363 1.185919
40
C26H14+:
C 0.260714 1.758029 -2.678612
C 0.053824 1.772419 -1.298556
C 0.001863 0.709564 -0.293826
C -0.001863 -0.709564 -0.293826
C -0.053824 -1.772419 -1.298556
C -0.260714 -1.758029 -2.678612
C -0.074096 1.352168 0.985751
C 0.074096 -1.352168 0.985751
C 0.057570 -0.726493 2.246179
C -0.057570 0.726493 2.246179
C 0.071733 -3.022490 -0.621128
C 0.148940 -2.757784 0.826104
C -0.071733 3.022490 -0.621128
C -0.148940 2.757784 0.826104
C 0.141265 -1.564949 3.368501
C -0.141265 1.564949 3.368501
C -0.279345 -2.968557 -3.386483
C 0.279345 2.968557 -3.386483
H -0.437168 -2.957845 -4.457758
H 0.132418 -1.150341 4.368698
H -0.132418 1.150341 4.368698
H 0.437168 2.957845 -4.457758
C -0.110146 -4.175494 -2.723141
C 0.236611 -2.949275 3.210677
C -0.236611 2.949275 3.210677
C -0.238959 3.565063 1.942810
C -0.056553 4.210605 -1.321994
C 0.110146 4.175494 -2.723141
C 0.056553 -4.210605 -1.321994
C 0.238959 -3.565063 1.942810
H -0.123700 -5.104246 -3.280836
H 0.160051 -5.162741 -0.814827
H 0.305336 -4.643687 1.867743
H 0.305236 -3.571745 4.095190
H -0.305236 3.571745 4.095190
H -0.305336 4.643687 1.867743
H -0.160051 5.162741 -0.814827
H 0.123700 5.104246 -3.280836
H 0.443934 0.836911 -3.211640
H -0.443934 -0.836911 -3.211640
40
TS3a:
C -2.525668 -0.999305 0.717178
C -1.146401 -1.463655 0.681026
C -0.010717 -0.691757 0.992236
C -0.007126 0.678486 1.001402
C -1.138722 1.460404 0.700428
C -2.520443 1.002977 0.730369
C 1.165550 -1.375842 0.570827
C 1.172752 1.361947 0.589163
C 2.409605 0.726428 0.349003
C 2.405720 -0.743670 0.339100
C -0.685656 2.641535 0.044178
C 0.809305 2.628039 0.069267
C -0.699572 -2.638353 0.009116
C 0.795468 -2.632983 0.034156
C 3.421851 1.575213 -0.166019
C 3.413473 -1.590742 -0.187389
C -3.402426 1.767485 -0.155547
C -3.411730 -1.747467 -0.178567
H -4.451416 1.500002 -0.209637
H 4.423121 1.198737 -0.337316
H 4.416666 -1.217217 -0.353843
H -4.459300 -1.473772 -0.228992
C -2.953325 2.882191 -0.809536
C 3.123414 2.882790 -0.527067
C 3.108194 -2.891805 -0.565823
C 1.788339 -3.411104 -0.530836
C -1.621969 -3.333869 -0.749867

C -2.968596 -2.855870 -0.847178
C -1.604226 3.351786 -0.705756
C 1.806279 3.408429 -0.485266
H -3.646985 3.452002 -1.416742
H -1.310232 4.226262 -1.275642
H 1.608067 4.381880 -0.918814
H 3.913841 3.504264 -0.930898
H 3.895327 -3.511942 -0.978061
H 1.585015 -4.377605 -0.977366
H -1.332693 -4.202324 -1.331258
H -3.665325 -3.413985 -1.461687
H -2.940620 -0.989534 1.724728
H -2.935641 0.982202 1.737649
40
C26H14+-IMa:
C -1.192748 -2.311252 -1.048189
C -1.560144 -0.869609 -1.049898
C -0.667175 0.149254 -1.352018
C 0.692167 -0.057902 -1.361314
C 1.245184 -1.296965 -1.068937
C 0.465338 -2.563865 -1.059114
C -1.173843 1.407065 -0.928724
C 1.555881 0.991207 -0.947105
C 1.110176 2.300573 -0.673146
C -0.354890 2.523754 -0.663191
C 2.517253 -1.068727 -0.453809
C 2.754511 0.415684 -0.458949
C -2.698264 -0.274225 -0.418334
C -2.482911 1.213481 -0.423541
C 2.105623 3.152301 -0.138059
C -1.044382 3.632091 -0.116522
C 1.089561 -3.548025 -0.114601
C -2.069931 -3.067177 -0.094526
H 0.602196 -4.505093 0.031213
H 1.889669 4.192887 0.072514
H -0.525629 4.560716 0.089266
H -1.888358 -4.126438 0.046074
C 2.308269 -3.327798 0.444308
C 3.359822 2.646003 0.192929
C -2.387944 3.521483 0.232087
C -3.110016 2.304214 0.151524
C -3.498531 -1.097759 0.338353
C -3.160307 -2.495226 0.480041
C 3.045808 -2.094463 0.294366
C 3.685559 1.269111 0.105409
H 2.748403 -4.103158 1.060717
H 3.967038 -1.972335 0.853342
H 4.625354 0.917734 0.515300
H 4.096327 3.322276 0.610596
H -2.884038 4.385468 0.658291
H -4.106232 2.247687 0.574671
H -4.334030 -0.708050 0.909426
H -3.803750 -3.105946 1.102834
H -1.483913 -2.710448 -2.034107
H 0.611229 -3.030001 -2.047745
40
TS4a:
C -2.375314 -0.830541 0.309105
C -1.128417 -1.416596 0.549219
C 0.034559 -0.693210 0.928472
C 0.032946 0.657857 0.962464
C -1.110911 1.415967 0.706792
C -2.459100 0.805007 0.582755
C 1.185625 -1.399273 0.552094
C 1.196852 1.373862 0.603113
C 2.417196 0.731899 0.312516
C 2.417919 -0.753889 0.295088
C -0.710714 2.668165 0.177437
C 0.799502 2.664011 0.169628
C -0.718333 -2.677359 0.044589
C 0.789679 -2.681037 0.071080
C 3.403930 1.600900 -0.211904
C 3.408711 -1.611874 -0.235602
C -3.395369 1.645609 -0.220188
C -3.357065 -1.623619 -0.307909
H -4.395086 1.285601 -0.422402
H 4.398684 1.237995 -0.442274
H 4.406340 -1.245973 -0.447815
H -4.350126 -1.249072 -0.524198
C -2.988747 2.877204 -0.647142
C 3.088949 2.926785 -0.507863
C 3.094505 -2.930584 -0.562896
C 1.784357 -3.469752 -0.477587
C -1.710556 -3.452712 -0.550149
C -3.013640 -2.927427 -0.683442
C -1.671343 3.431091 -0.471580
C 1.784275 3.464420 -0.387622
H -3.703435 3.463317 -1.214570
H -1.439796 4.382292 -0.933872
H 1.582670 4.459443 -0.767146
H 3.865956 3.559118 -0.921124
H 3.876116 -3.555797 -0.978506
H 1.590115 -4.455203 -0.884804
H -1.497680 -4.433433 -0.960128
H -3.771768 -3.540469 -1.155594
H -2.888572 -0.004095 1.497240
H -2.928145 0.978557 1.736870
38
C26H12+:
C 2.394405 0.755615 0.233950
C 1.162785 1.401370 0.474930
C 0.000000 0.682065 0.739638
C 0.000000 -0.682065 0.739638
C 1.162785 -1.401370 0.474930
C 2.394405 -0.755615 0.233950
C -1.162785 1.401370 0.474930
C -1.162785 -1.401370 0.474930
C -2.394405 -0.755615 0.233950
C -2.394405 0.755615 0.233950
C 0.768529 -2.721421 0.115327
C -0.768529 -2.721421 0.115327
C 0.768529 2.721421 0.115327
C -0.768529 2.721421 0.115327
C -3.397382 -1.634694 -0.21516
C -3.397382 1.634694 -0.215186
C 3.397382 -1.634694 -0.215186
C 3.397382 1.634694 -0.215186
H 4.401514 -1.288272 -0.428552
H -4.401514 -1.288272 -0.428552
H -4.401514 1.288272 -0.428552
H 4.401514 1.288272 -0.428552
C 3.086610 -2.982447 -0.452492
C -3.086610 -2.982447 -0.452492
C -3.086610 2.982447 -0.452492
C -1.780766 3.540475 -0.344058
C 1.780766 3.540475 -0.344058
C 3.086610 2.982447 -0.452492
C 1.780766 -3.540475 -0.344058

C -1.780766 -3.540475 -0.344058
H 3.882329 -3.629707 -0.803318
H 1.616177 -4.562824 -0.662686
H -1.616177 -4.562824 -0.662686
H -3.882329 -3.629707 -0.803318
H -3.882329 3.629707 -0.803318
H -1.616177 4.562824 -0.662686
H 1.616177 4.562824 -0.662686
H 3.882329 3.629707 -0.803318
65
C39H26+:
C 0.000042 -0.024631 0.000162
C 1.118150 0.852629 0.704136
C -1.118151 0.852669 -0.703642
C 0.643344 -0.997268 -0.992696
C -0.643164 -0.997595 0.992766
C 1.909106 1.789447 -0.212510
C 2.238886 0.015822 1.326101
C -1.909619 1.788820 0.213248
C -2.238469 0.015809 -1.326272
C 0.396547 -2.335536 -0.607131
C -0.396333 -2.335736 0.606782
C 3.284729 1.446104 -0.187082
C 3.484578 0.362429 0.753109
C -3.285126 1.445038 0.187339
C -3.484404 0.361734 -0.753403
C 1.367680 -0.731562 -2.146042
C -1.367464 -0.732267 2.146220
C 1.499175 2.873749 -0.979566
C 2.194243 -0.922029 2.347605
C -1.500234 2.872917 0.980889
C -2.193268 -0.921557 -2.348194
C 0.882712 -3.406414 -1.370740
C -0.882445 -3.406866 1.370074
C 4.225296 2.151246 -0.949692
C 4.672671 -0.262280 1.162408
C -4.226103 2.149509 0.950062
C -4.672193 -0.263176 -1.163272
C 1.852283 -1.803370 -2.904385
C -1.852012 -1.804325 2.904246
C 1.611975 -3.130238 -2.518750
C -1.611683 -3.131068 2.518190
C 2.442522 3.579240 -1.736680
C 3.382461 -1.539565 2.757797
C -2.443991 3.577737 1.738115
C -3.381186 -1.539293 -2.758955
C 3.794398 3.214961 -1.729901
C 4.611290 -1.220122 2.162595
C -3.795740 3.213002 1.730867
C -4.610260 -1.220532 -2.163892
H 0.622577 1.427636 1.490776
H -0.622556 1.428175 -1.489903
H 1.554698 0.282458 -2.475843
H -1.554495 0.281644 2.476344
H 0.468659 3.200917 -1.005759
H 1.267189 -1.175398 2.842853
H -0.469839 3.200431 1.007462
H -1.266008 -1.174395 -2.843330
H 0.694301 -4.431381 -1.073362
H -0.694002 -4.431735 1.072377
H 5.274447 1.881351 -0.920908
H 5.623275 0.008720 0.718296
H -5.275157 1.879273 0.920913
H -5.622991 0.007303 -0.719259
H 2.419888 -1.604988 -3.806206
H -2.419592 -1.606240 3.806148
H 1.999332 -3.941705 -3.123278
H -1.998997 -3.942734 3.122478
H 2.119448 4.424314 -2.333444
H 3.351896 -2.271547 3.556571
H -2.121340 4.422650 2.335337
H -3.350191 -2.270891 -3.558066
H 4.505235 3.776879 -2.323824
H 5.515171 -1.713522 2.499187
H -4.506901 3.774405 2.324888
H -5.513898 -1.714074 -2.500926
63
C39H24+:
C 0.040402 -0.493059 0.007883
C 1.231741 0.425205 0.148846
C -1.292095 0.199971 -0.152191
C 0.166483 -1.463027 1.215020
C 0.089439 -1.496443 -1.177054
C 1.250955 1.631296 0.951046
C 2.573349 0.214240 -0.355918
C -1.517701 1.369778 -0.975626
C -2.579208 -0.235269 0.351074
C 0.281281 -2.789689 0.763918
C 0.215435 -2.811858 -0.696754
C 2.578397 2.149595 0.962486
C 3.407909 1.265086 0.134040
C -2.915685 1.645524 -1.002611
C -3.582430 0.643042 -0.161545
C 0.208636 -1.164287 2.570920
C -0.008014 -1.240342 -2.538858
C 0.245341 2.289931 1.674262
C 3.136796 -0.791543 -1.158281
C -0.637858 2.182336 -1.706191
C -2.960636 -1.310665 1.169794
C 0.408607 -3.832288 1.681282
C 0.277092 -3.880419 -1.590460
C 2.892685 3.280540 1.689249
C 4.751255 1.313535 -0.175540
C -3.418285 2.690653 -1.751579
C -4.915264 0.457969 0.141822
C 0.334760 -2.212976 3.484984
C 0.055377 -2.314942 -3.429273
C 0.573161 3.423116 2.420123
C 4.497206 -0.734315 -1.465712
C -1.154145 3.227107 -2.474115
C -4.311851 -1.490165 1.470749
C 0.432908 -3.534569 3.043337
C 0.197992 -3.622356 -2.958473
C 1.877360 3.916947 2.423645
C 5.295559 0.302557 -0.986771
C -2.524832 3.483235 -2.492575
C -5.277456 -0.619546 0.969189
H 0.143710 -0.144650 2.928829
H -0.129095 -0.233947 -2.919202
H -0.780501 1.945288 1.659859
H 2.542625 -1.606957 -1.541390
H 0.432323 2.023248 -1.679781
H -2.232822 -1.999707 1.569851
H 0.485905 -4.859973 1.345437
H 0.385140 -4.897595 -1.231870
H 3.901620 3.676043 1.705587
H 5.385720 2.108473 0.198924
H -4.480896 2.901982 -1.780260

H -5.678071 1.121181 -0.249252
H 0.362061 -1.996395 4.546242
H -0.012533 -2.130733 -4.494808
H -0.196558 3.932821 2.986568
H 4.935378 -1.507475 -2.084928
H -0.481844 3.854593 -3.046280
H -4.610925 -2.317422 2.102719
H 0.534621 -4.335365 3.766317
H 0.240919 -4.444357 -3.663309
H 2.111112 4.807480 2.995298
H 6.349442 0.329338 -1.237857
H -2.907254 4.308746 -3.081433
H -6.321250 -0.775563 1.215358
61
C39H22+:
C 0.670424 -0.594494 0.274807
C -0.071577 0.388230 1.142676
C 2.094941 -0.111870 -0.010820
C 0.974856 -2.055052 0.677177
C 0.488364 1.694663 1.299533
C -1.369814 0.389886 1.803994
C 2.921949 -1.197834 -0.309187
C 2.219161 -2.420767 0.116528
C -0.395550 2.515273 2.045216
C -1.569061 1.687664 2.371501
C 2.610158 1.169779 0.186093
C 1.742286 2.147178 0.846520
C 4.252099 -0.975512 -0.658944
C 2.707044 -3.715823 0.256285
C -0.042578 3.814863 2.332616
C -2.710025 1.980913 3.090571
C 3.963070 1.383056 -0.147887
C 0.820908 -4.235201 1.679051
C 4.748969 0.332622 -0.611914
C 1.985985 -4.630642 1.026009
C 2.078639 3.481792 1.143720
C -3.513629 -0.278926 2.687258
C 1.204193 4.287490 1.862585
C -3.687106 0.983677 3.248838
H 4.912896 -1.797913 -0.906406
H 3.658544 -3.999598 -0.178391
H -0.687807 4.471911 2.903432
H -2.859685 2.960963 3.528391
H 4.411635 2.359084 -0.011879
H 0.308723 -4.928020 2.336118
H 5.784165 0.518893 -0.872027
H 2.362320 -5.638142 1.157686
H 3.027433 3.892171 0.822555
H -4.281184 -1.032921 2.812142
H 1.490910 5.310217 2.078758
H -4.586766 1.202199 3.811907
C -0.255279 -0.456297 -0.972699
C -0.276279 0.652805 -1.928747
C -1.412967 -1.296913 -1.282320
C 0.631436 1.677627 -2.238851
C -1.477695 0.565429 -2.692119
C -1.818860 -2.567211 -0.846238
C -2.181906 -0.652917 -2.293625
C 0.316139 2.607717 -3.231628
H 1.591322 1.746694 -1.759732
C -1.790114 1.491162 -3.666662
C -2.982940 -3.139289 -1.363411
H -1.230488 -3.135453 -0.146332
C -3.336842 -1.217266 -2.798018
C -0.885556 2.531634 -3.929308
H 1.027112 3.390192 -3.467537
H -2.710488 1.415100 -4.233780
C -3.745895 -2.469615 -2.316338
H -3.283654 -4.124376 -1.027579
H -3.913770 -0.715616 -3.566069
H -1.115210 3.263649 -4.694595
H -4.646981 -2.927618 -2.707108
C 0.308926 -2.942374 1.507404
H -0.584404 -2.653277 2.044216
C -2.359450 -0.585773 1.962473
H -2.261420 -1.566044 1.521077
59
C39H20+-1:
C -0.462176 0.000034 -0.805901
C -0.090768 0.000029 0.625070
C -1.227924 -1.165088 -1.269085
C -1.227935 1.165155 -1.269074
C -0.445812 -1.159560 1.425488
C -0.445821 1.159610 1.425498
C -2.083207 -0.745938 -2.314964
C -2.083215 0.746006 -2.314956
C -0.579121 -0.741378 2.778208
C -0.579127 0.741413 2.778214
C -1.424944 -2.336519 -0.526716
C -1.424979 2.336573 -0.526690
C -0.986963 -2.341366 0.909710
C -0.986994 2.341411 0.909735
C -2.949615 -1.690488 -2.867159
C -2.949634 1.690551 -2.867143
C -0.967720 -1.701355 3.718315
C -0.967733 1.701376 3.718332
C -2.307052 -3.270490 -1.106209
C -2.307100 3.270538 -1.106172
C -2.998598 -2.963796 -2.284334
C -2.998637 2.963851 -2.284303
C -1.368484 -3.285784 1.883499
C -1.368524 3.285816 1.883533
C -1.298789 -2.978169 3.252727
C -1.298819 2.978191 3.252758
H -3.618920 -1.443494 -3.682760
H -3.618934 1.443557 -3.682748
H -1.070601 -1.463720 4.770357
H -1.070610 1.463730 4.770372
H -2.510123 -4.215461 -0.616414
H -2.510185 4.215501 -0.616365
H -3.667178 -3.707086 -2.702445
H -3.667227 3.707136 -2.702406
H -1.778230 -4.245522 1.591438
H -1.778285 4.245551 1.591482
H -1.601072 -3.734800 3.967107
H -1.601110 3.734812 3.967146
C 1.035454 0.000019 -0.477458
C 1.964048 -1.185758 -0.562132
C 1.964112 1.185751 -0.562139
C 1.759840 -2.543922 -0.773201
C 3.304700 -0.717353 -0.410150
C 1.759992 2.543926 -0.773228
C 3.304740 0.717269 -0.410156
C 2.855393 -3.413272 -0.761289
H 0.783341 -2.951165 -0.971382
C 4.396344 -1.599242 -0.380576
C 2.855597 3.413209 -0.761323
H 0.783523 2.951230 -0.971424

C 4.396436 1.599092 -0.380588
C 4.164046 -2.952020 -0.545912
H 2.686513 -4.470689 -0.928682
H 5.404204 -1.222902 -0.253839
C 4.164222 2.951882 -0.545937
H 2.686782 4.470635 -0.928732
H 5.404274 1.222693 -0.253847
H 4.988008 -3.654974 -0.535036
H 4.988227 3.654787 -0.535069
59
C39H20+-2:
C 0.000830 0.986755 -0.000134
C 0.523357 -0.081925 -0.952971
C 1.141238 1.939860 0.310022
C -1.138083 1.941499 -0.310721
C 1.901103 -0.446529 -0.783974
C -0.056083 -1.001582 -1.912723
C 0.708674 3.266914 0.208707
C -0.703541 3.267922 -0.209704
C 2.182885 -1.619223 -1.523388
C 0.946138 -1.966447 -2.250952
C 2.498146 1.611637 0.380693
C 2.884488 0.270272 -0.080041
C 1.619253 4.304510 0.422402
C -1.612548 4.306826 -0.423743
C 3.456287 -2.148536 -1.491011
C 0.680909 -2.959377 -3.172168
C 3.401087 2.661767 0.623600
C -3.396811 2.666692 -0.624804
C 2.952987 3.981939 0.681862
C -2.946730 3.986184 -0.683292
C 4.175082 -0.290167 -0.054434
C -1.556965 -2.045496 -3.478775
C 4.439750 -1.477516 -0.729588
C -0.586052 -2.998409 -3.780578
H 1.312482 5.341974 0.361593
H -1.304230 5.343845 -0.363178
H 3.718126 -3.047527 -2.036178
H 1.432244 -3.693964 -3.437704
H 4.462438 2.460693 0.703945
H -4.458449 2.467179 -0.705246
H 3.668256 4.775613 0.861820
H -3.660789 4.780883 -0.863538
H 4.978092 0.206935 0.475749
H -2.516625 -2.079833 -3.979856
H 5.442168 -1.888333 -0.693553
H -0.803338 -3.772528 -4.507140
C -0.523447 -0.080680 0.953142
C 0.054402 -1.000731 1.913487
C -1.901687 -0.443335 0.783995
C 1.299985 -1.038664 2.546436
C -0.949302 -1.964007 2.251860
C -2.883856 0.274608 0.079528
C -2.185352 -1.615315 1.523813
C 1.553320 -2.046091 3.480466
H 2.054014 -0.292304 2.342299
C -0.685765 -2.956906 3.173595
C -4.175244 -0.283986 0.053790
C -3.459499 -2.142823 1.491288
C 0.580958 -2.997482 3.782398
H 2.512778 -2.081572 3.981855
H -1.438230 -3.690292 3.439252
C -4.441791 -1.470699 0.729326
H -4.977403 0.214079 -0.476776
H -3.722778 -3.041221 2.036741
H 0.796918 -3.771587 4.509371
H -5.444788 -1.880092 0.693185
C -2.495468 1.615280 -0.381514
C -1.301913 -1.038018 -2.545268
H -2.054814 -0.290497 -2.341203

## REFERENCES

Becke, A. D., 1992, JChPh, 96, 2155
Dibben, Ma. J., Kage, D., Szczepanski, J., Eyler, J. R., and Vala, M. 2001, JPCA, 105, 6024
Frisch, M. J., et al., Gaussian 16 revision e.01, Gaussian Inc.
Lang, M., Holzmeier, F., Fischer, I,, et al. 2013, JPCA, 117, 5260
Lee, C., Yang, W., Parr, R. G. 1988, PhReB, 37, 785
Stein, T., Bandyopadhyay, B., Troy, T.P., et al., 2017, Proc Nat Acad Sci, 114, E4125
Zhen, J., Paardekooper, D. M., Candian, A., Linnartz, H. Tielens, A. G. G. M. 2014a, CPL, 592, 211
B. West, S. Rodriguez Castillo, A. Sit, S. Mohamad, B. Lowe, C. Joblin, A. Bodi, P.M. Mayer, Phys. Chem. Chem. Phys. 20, 7195 (2018)
O'Reilly, R. J., Karton, F. 2016, Inter. J. Quantum. Chem., 116, 52
